# Supplementary material for: Scalable all-optical cold damping of levitated nanoparticles
Source: arXiv:2205.04455 source file (2022-05-09)
Supplement: Supplementary file 1 [file Contribution_to_linear_feedback_from_tweezer_motion.tex]

\centerline{\textbf{Contribution from tweezer motion}}
\label{sec:tweezer motion}
\vspace{1mm} 

\begin{figure}
    \includegraphics[width = 8cm]{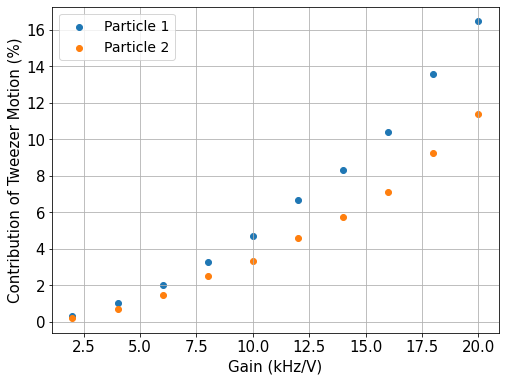}
    \caption{\textbf{Contribution from tweezer motion in the measured PSD.}
    }
    \label{fig:tweezermotion}
\end{figure}
As pointed out in the main text, the signal measured by the QPD has contributions from both the particle motion ($\Omega_y$) and the tweezer modulation $\Delta\omega$.
Here we investigate our linear feedback loop carefully to estimate the relative contribution of the tweezer modulation to the total signal measured by the QPD.

First, we measure the QPD signal (both the in-loop one and out-of-loop one) at different level of frequency modulation at the AOD. With no particle trapped and no feedback loop, we use an external source (Zurich Instruments MFLI) to send a $75\,$kHz sin signal at different voltage amplitudes $V_{\text{in}}$ as input to the function generator driving the AOD. This simulates the contribution of the tweezer modulation to the power spectral density for different voltages. At different amplitude of frequency modulation at the AOD $\Delta\omega=G_{\text{AOD}}V_{\text{in}}$, we measure the corresponding PSD area at the QPD $A_{\text{tweezer}}(\Delta \omega)$. We then fit the data $A_{\text{tweezer}}(\Delta\omega)$ with a quadratic function $A_{\text{tweezer}}^{\text{fit}}(\Delta \omega)=k\Delta \omega^2$. 

Then, we characterize the contribution of the tweezer modulation on the measured signal $V_{\text{il}}$. At each gain factor $G_{\text{FG}}$ at the RF generator, we measure the in-loop voltage and calculate the frequency modulation $\Delta\omega=G_{\text{FG}}V_{\text{il}}$. Then, we estimate the PSD area contributed by this frequency modulation with $A_{\text{tweezer}}^{\text{fit}}(G_{\text{FG}}V_{\text{il}})$. By comparing the PSD area of the tweezer motion to the total PSD, we find out the relative contribution of the tweezer motion: $A_{\text{tweezer}}^{\text{fit}}(G_{\text{FG}}V_{\text{il}})/A_{\text{total}}$ (see Fig.\ref{fig:tweezermotion}). As the particle motion is cooled closer to the noise floor by increasing the feedback gain $G_{\text{var}}$, we find that the relative contribution of the tweezer motion to the overall signal at the QPD rises. The maximum relative contribution of the tweezer motion is about $15\%$. So, the tweezer modulation is small and the extracted temperatures from PSD are reliable.

We can do a simple scaling analysis of relative quantities on the gain factor at RF function generator $G_{\text{FG}}$. The PSD area contributed by the particle motion, which is proportional to the particle energy is $A_{\text{particle}}\propto E=E_0\gamma_{\text{gas}}/\gamma_{\text{fb}} \propto 1/G_{\text{FG}}$. The in-loop voltage is proportional to the square root of the PSD area: $V_{\text{il}} \propto \sqrt{A_{\text{particle}}} \propto 1/\sqrt{G_{\text{FG}}}$. The frequency modulation is the product of in-loop voltage and the gain at function generator: $\Delta \omega=G_{\text{FG}}V_{\text{il}} \propto \sqrt{G_{\text{FG}}}$. The PSD area contributed by tweezer motion is a quadratic function of frequency modulation:
$A_{\text{tweezer}}\propto \Delta \omega^2\propto G_{\text{FG}}$. Finally, we get the relative contribution of the tweezer motion to the particle signal (as well as the overall signal, when the tweezer motion part is small) is quadratic in the gain at function generator
$A_{\text{tweezer}}/A_{\text{particle}} \propto G_{\text{FG}}^2$. This analysis agrees with the result in Fig.\ref{fig:tweezermotion}.

\vspace{5mm}
